# Supplementary material for: Quaternion Backpropagation
Source: arXiv:2212.13082 source file (2022-12-26)
Supplement: Supplementary file 1 [file appendix.tex]

\appendix
\section{Using the Product Rule}

Initially, we use the product rule as this is the most intuitive way to obtain the derivative of the loss $\loss$ with respect to $w_i$ and $b_i$. Hence, we derive with respect to the first weight $w_1^*$ 

\begin{equation}
    \frac{\partial \loss}{\partial w_1^*}
    = \frac{\partial e^* e}{\partial w_1^*} 
    = \frac{\partial (d - y)^*(d - y)}{\partial w_1^*}
    = e^* \frac{\partial e}{\partial w_1^*} + \frac{\partial e^*}{\partial w_1^{e^*}} e
\end{equation}

Because we derive with respect to $w_1^*$ we can simplify $y = w_1 a_1$, omitting all biases and all other weights for now. Then, we can calculate the first respective partial derivatives:
\begin{equation}
    \frac{\partial e}{\partial w_1^*} 
    = \frac{\partial (d - w_1 a_1 )}{\partial w_1^*} 
    = -\frac{\partial (w_1 a_1)}{\partial w_1^*}
    = \frac{1}{2} a_1^*
\end{equation}

The second partial derivative is derived as follows:

\begin{equation}
\begin{aligned}
    \frac{\partial e^*}{\partial w_1^{e^*}}
    &= \frac{\partial (d - a_1 w_1)^*}{\partial w_1^{e^*}}
    = - \frac{\partial (a_1 w_1)^*}{\partial w_1^{e^*}}
    = - \frac{\partial w_1^* a_1^*}{\partial w_1^{e^*}} \\
    &= - \frac{1}{4} \left( a_1^* - a_1^*ii^e - a_1^*jj^e - a_1^*kk^e \right) \\
    &= - \frac{1}{4} \left( a_1^* ee^{-1} - a_1^*ieie^{-1} - a_1^*jeje^{-1} - a_1^*keke^{-1} \right) \\
    &= - \frac{1}{4} a_1^*\left( e - iei - jej - kek \right) e^{-1} \\
    &= - \frac{1}{4} a_1^*\left(e + e^i + e^j + e^k \right) e^{-1} \\
    &= - a_1^* e_0 e^{-1} \\
\end{aligned}
\end{equation}

Putting everyting together, we obtain

\begin{equation}
\begin{aligned}
    \frac{\partial \loss}{\partial w_1^*}
    &= e^* \frac{\partial e}{\partial w_1^*} + \frac{\partial e^*}{\partial w_1^{e^*}} e \\
    &= e^* \frac{1}{2}a_1^* - a_1^* e_0 e^{-1} e \\
    &= \left(\frac{1}{2}e_0 - \frac{1}{2}e_1 - \frac{1}{2}e_2 - \frac{1}{2}e_3  - e_0 \right)a_1^*
    &= -\frac{1}{2}ea_1^* .
\end{aligned}
\end{equation}

Likewise, we can also do the same derivations with respect to $b_1$:
\begin{equation}
    \frac{\partial \loss}{\partial b_1^*}
    = \frac{\partial e^* e}{\partial b_1^*} 
    = e^* \frac{\partial e}{\partial b_1^*} + \frac{\partial e^*}{\partial b_1^{e^*}} e
\end{equation}

\begin{equation}
\begin{aligned}
    \frac{\partial e}{\partial b_1^*}
    = \frac{\partial \left(d - \left(w_1 a_1  + b_1\right) \right)}{\partial b_1^*} = -\frac{\partial b}{\partial b_1^*} = \frac{1}{2}
\end{aligned}
\end{equation}

\begin{equation}
\begin{aligned}
    \frac{\partial e^*}{\partial b_1^{e^*}}
    &= \frac{\partial \left(d - \left(w_1 a_1  + b_1\right) \right)^*}{\partial b_1^{e^*}}
    = - \frac{\partial b^*}{\partial b_1^{e^*}} \\
    &= -\frac{1}{4}(-e+iei + jej + kek)e^{-1} \\
    &= \frac{1}{4} \left(e + e^i + e^j + e^k \right) e^{-1} \\
    &= -e_0 e^{-1}
\end{aligned}
\end{equation}

Combining the respective partial derivatives yields
\begin{equation}
\begin{aligned}
    \frac{\partial \loss}{\partial b_1^*}
    &= e^* \frac{\partial e}{\partial b_1^*} + \frac{\partial e^*}{\partial b_1^{e^*}} e \\
    &= \frac{1}{2}e^* + e_0 e^{-1} e \\
    &= \frac{1}{2} (e_0 - e_1i - e_2j - e3k) - e_0 \\
    &= -\frac{1}{2}e
\end{aligned}
\end{equation}
as the derivation of $\loss$ with respect to $b_1$.

Same calculations can be done for all remaining weights and biases $i \in \{2, \dots, n\}$. \\

At this point, we will dispense with the calculation for the derivative with respect to the activation of the previous layer as it can be done analogous to the previous calculations and will be calculated using the chain rule later on.
